# Supplementary material for: The multi-modal universe of fast-fashion: the Visuelle 2.0 benchmark
Source: arXiv:2204.06972 source file (2022-11-30)

GRU

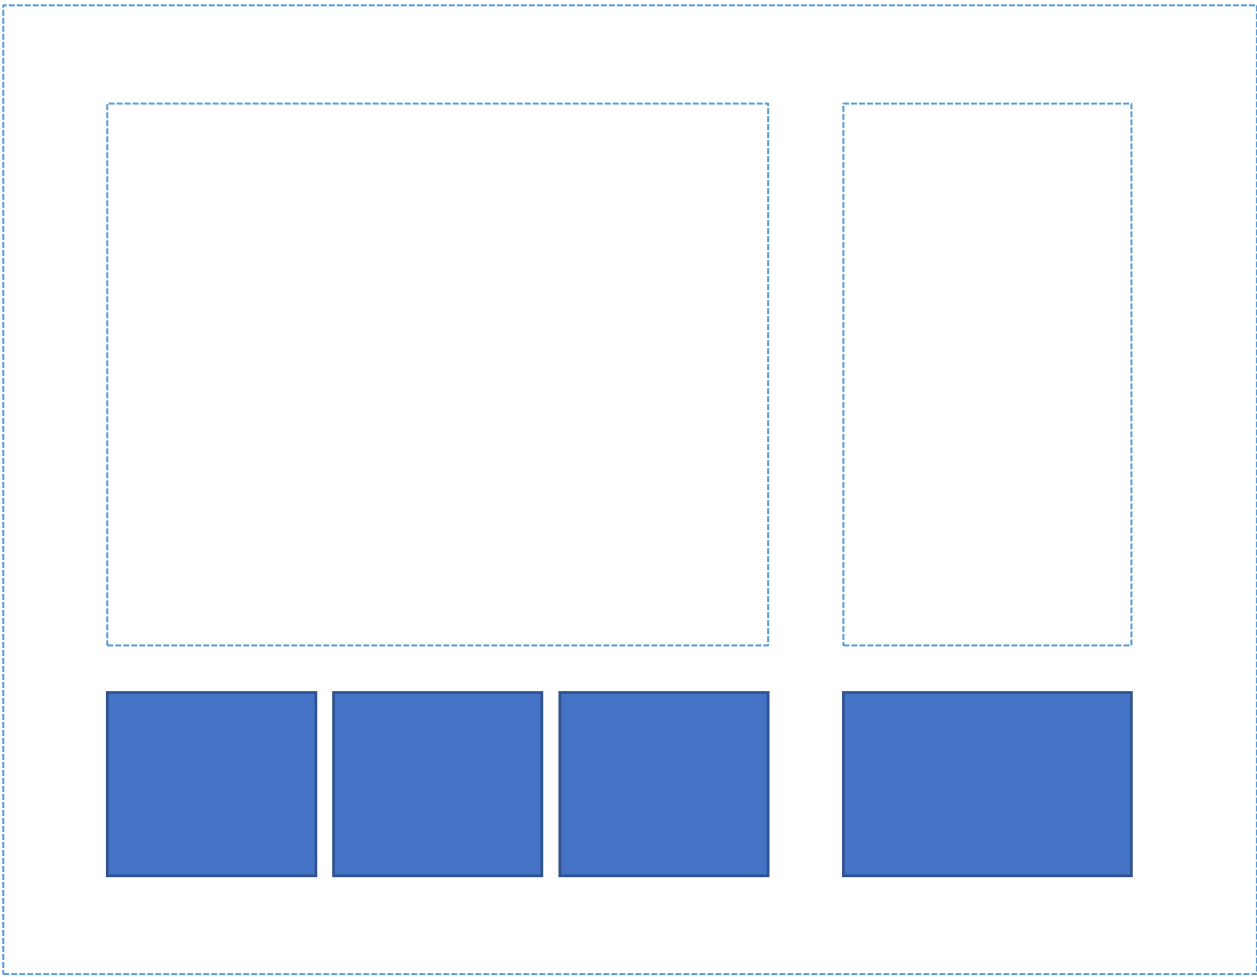

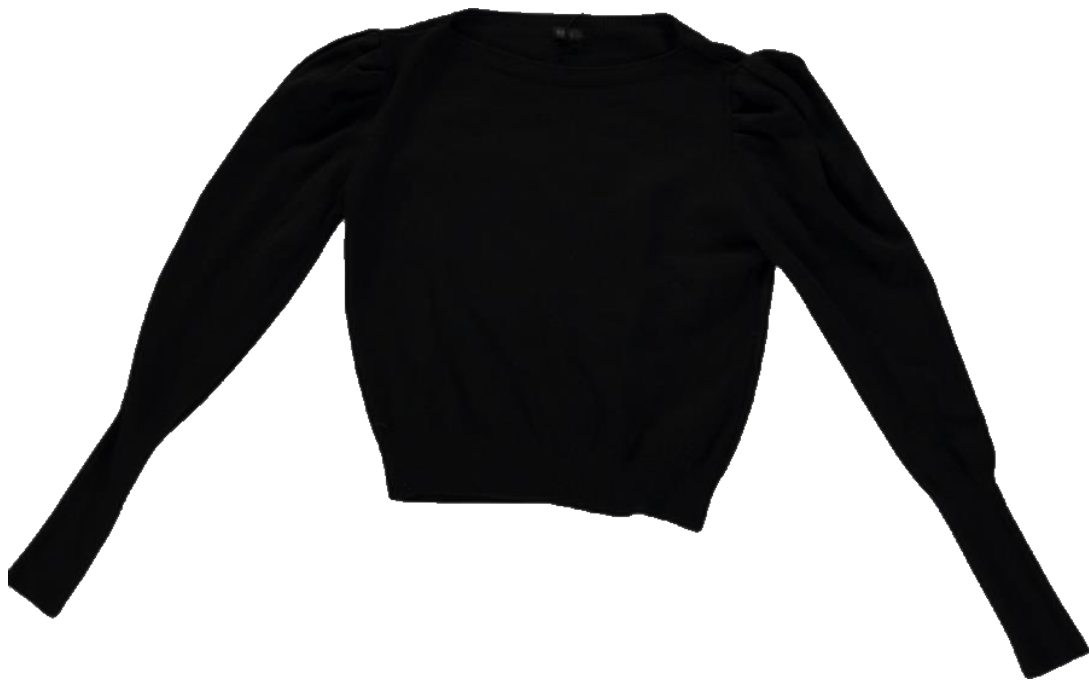

**Category:** Long sleeve

**Color:** Black

**Fabric:** Acrylic

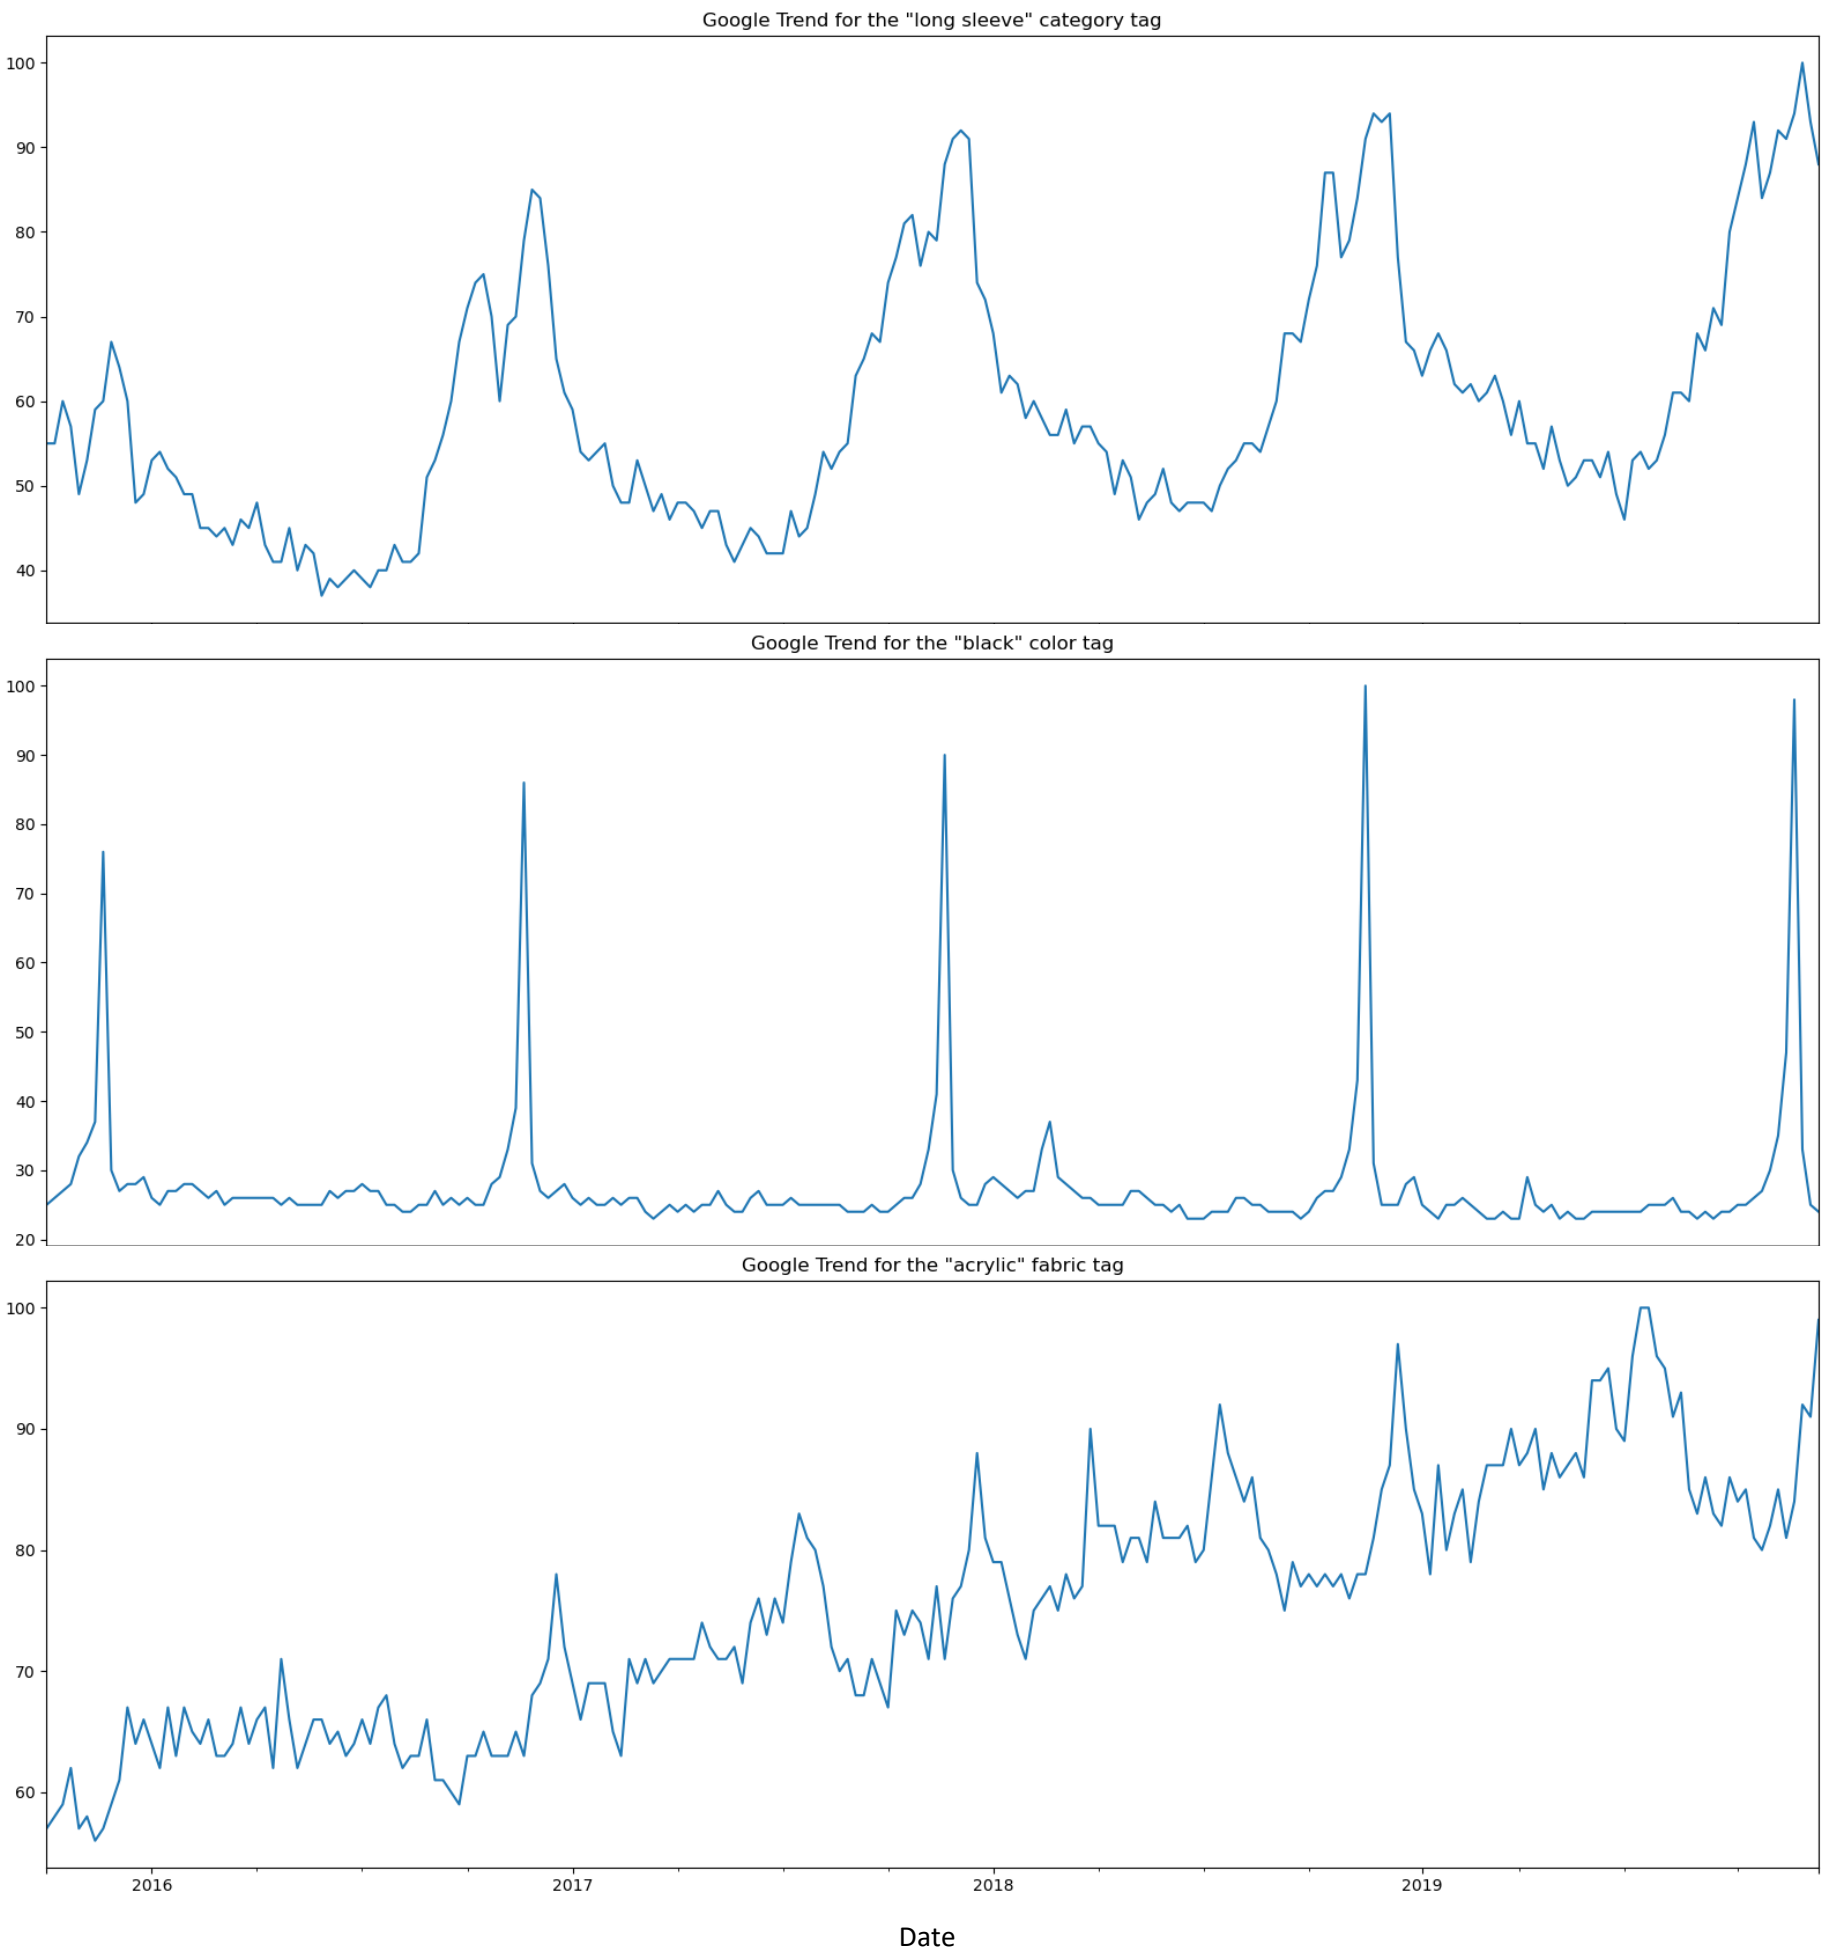

Supplement: Supplementary file 1 [file trends.pdf]
